# Supplementary material for: Bayesian analysis of flexible Heckman selection models using Hamiltonian Monte Carlo
Source: arXiv:2510.20942 ancillary file (2025-10-23)
Supplement: Supplementary file 1 [file supplementary.pdf]

# Supplement to: Bayesian analysis of flexible Heckman selection models using Hamiltonian Monte Carlo

Heeju Lim

Department of Statistics, University of Connecticut

Victor E. Lachos

Department of Applied Mathematics and Statistics,  
University of São Paulo, São Carlos, Brazil

Victor H. Lachos

Department of Statistics, University of Connecticut

October 22, 2025

## S.1 Prior Sensitivity Analysis

To validate the robustness and flexibility of the SL models, we generated synthetic sample selection data from a bivariate Student-t error structure with degrees of freedom  $\nu = 5$ . This design allows us to evaluate model performance under controlled heavy-tailed error settings.

### $\nu$ parameter for SLt model

To evaluate the robustness of our Bayesian Heckman selection model to prior choices for the degrees of freedom parameter  $\nu$ , we conducted a sensitivity analysis using four distinct prior distributions: (i)  $\mathcal{T}(0, 5, 4)$ , (ii)  $\mathcal{G}(2, 0.1)$ , (iii) Uniform(2, 30), and (iv) Cauchy(0, 5). The four priors for the degrees of freedom parameter  $\nu$  were truncated to  $[2, \infty)$  to ensure finite variance of the  $t$ -distribution, and were selected to represent a broad range of assumptions regarding tail heaviness:

- (i)  $\mathcal{T}(0, 5, 4)$  **truncated to**  $[2, \infty)$  : A heavy-tailed Student-t prior centered at zero with scale 5, ensuring support over positive values and allowing substantial mass on moderate  $\nu$  values.
- (ii)  $\mathcal{G}(2, 0.1)$  **truncated to**  $[2, \infty)$  : A positively skewed gamma prior with mean 20 and variance 200, placing more weight on moderate to large values of  $\nu$ .

- (iii) **Uniform(2, 30)**: A non-informative flat prior over the interval  $[2, 30]$ , treating all admissible degrees of freedom equally likely.
- (iv) **Cauchy(0, 5) truncated to  $[2, \infty)$** : A heavy-tailed prior that decays slowly, maintaining substantial probability mass for large  $\nu$  values while ensuring finite variance through the truncation at 2.

Figure S.1.1 illustrates the posterior densities of  $\nu$  under each prior scenario. Despite the notable differences in prior shapes were consistently concentrated between approximately 4 and 8. This suggests that the posterior inference for  $\nu$  was largely driven by the data rather than dominated by prior assumptions.

These findings indicate that the model yields stable and robust estimates for  $\nu$ , supporting the validity of the  $t$ -error specification regardless of moderate prior variation.

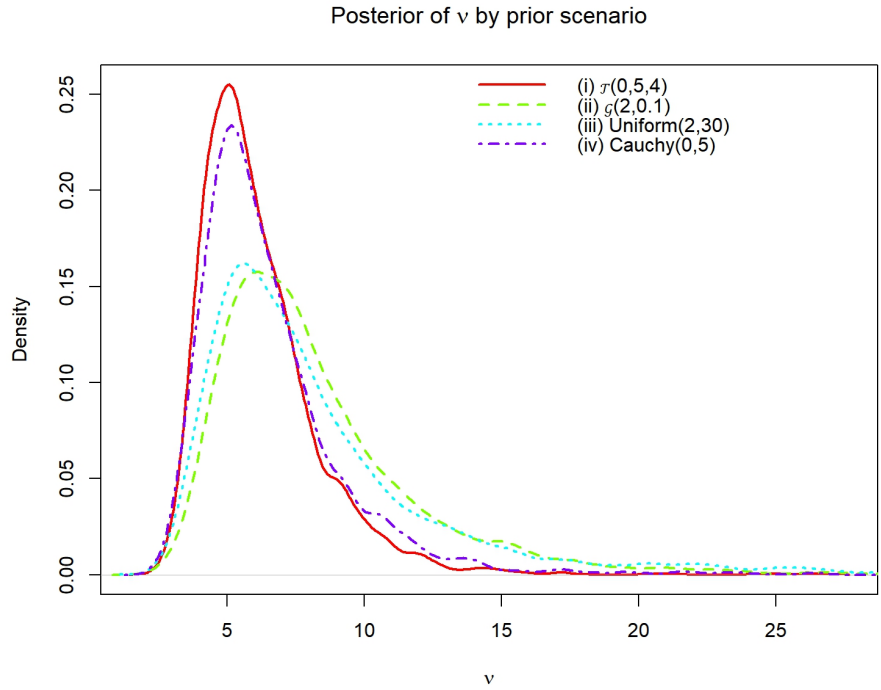

Figure S.1.1: Posterior densities of the degrees of freedom parameter  $\nu$  truncated to  $[2, \infty)$  under four prior specifications:  $\mathcal{T}(0, 5, 4)$ ,  $\mathcal{G}(2, 0.1)$ ,  $\text{Uniform}(2, 30)$ , and  $\text{Cauchy}(0, 5)$

## Contamination Parameter $\nu_1$ for SLcn Model

As empirical results showed a negligible impact of  $\nu_2$  on posterior inference, we omitted a separate sensitivity analysis for this parameter, focusing instead on  $\nu_1$ , which directly governs the contamination probability.

To assess the robustness of inference regarding the contamination probability parameter  $\nu_1$  in the SLcn model, we conducted a prior sensitivity analysis under four distinct specifications: (i)  $\text{Uniform}(0, 1)$ , (ii)  $\text{Beta}(2, 2)$ , (iii)  $\text{Log-Uniform}(0, 1)$ , and (iv)  $\mathcal{N}(0.5, 0.3)$ . The four priors for the contamination probability parameter  $\nu_1$  were truncated to  $[0, 1]$  and were selected to span a broad range of plausible prior beliefs:

- (i) **Uniform**(0, 1): A flat, non-informative prior assigning equal probability across the entire admissible range of contamination probabilities.
- (ii) **Beta**(2, 2): A symmetric prior with mean 0.5, favoring moderate values while down-weighting extreme probabilities near 0 or 1.
- (iii) **Log-Uniform**(0, 1): An improper prior on the unit interval defined by  $\log \nu_1 \sim \text{Uniform}(-\infty, 0)$ . Equivalently, it has density  $f(\nu_1) \propto \nu_1^{-1}$  for  $0 < \nu_1 < 1$ , which allocates relatively more prior mass to small values of  $\nu_1$ .
- (iv)  $\mathcal{N}(0.5, 0.3)$  **truncated to**  $[0, 1]$  : A bell-shaped prior centered at 0.5, placing most weight around moderate contamination levels while ensuring support within the valid range.

Together, these priors represent flat, symmetric, small-value-favoring, and centered informative specifications, allowing us to evaluate posterior robustness under diverse assumptions. These priors reflect a range of assumptions from noninformative to mildly informative.

Figure S.1.2 shows the resulting posterior densities of  $\nu_1$  under each scenario. Despite notable differences in prior shape, the posterior distributions exhibit strong concentration within a consistent range, typically between 0.3 and 0.7. This suggests that the posterior inference for  $\nu_1$  is primarily data-driven, and the estimation is robust to moderate variations in the prior specification.

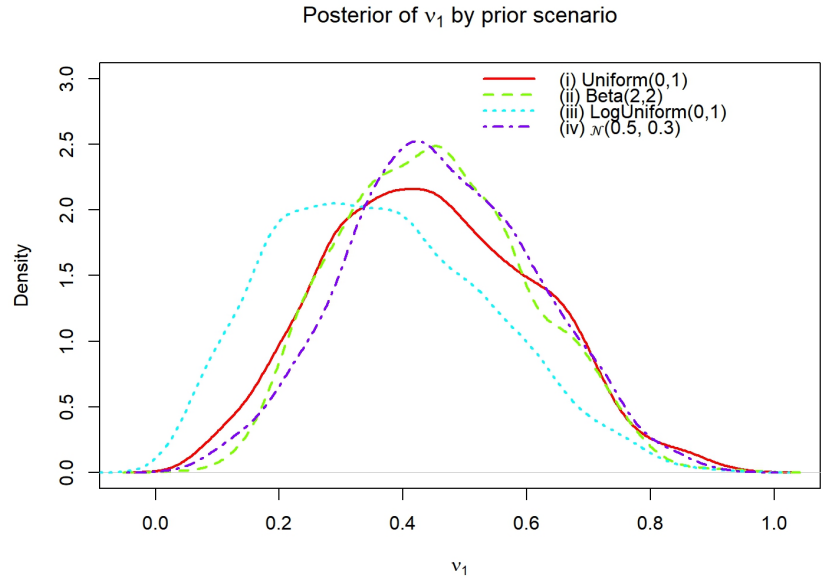

Figure S.1.2: Posterior densities of the contamination parameter  $\nu_1$  truncated to  $[0, 1]$  under four prior specifications: Uniform(0, 1), Beta(2, 2), Log-uniform(0, 1), and  $\mathcal{N}(0.5, 0.3)$ .

## S.2 Pseudo-code for SL Models

### Hamiltonian Monte Carlo (HMC) Algorithm

Hamiltonian Monte Carlo (HMC) is a Markov Chain Monte Carlo (MCMC) method used in Bayesian inference to sample from complex posterior distributions. Unlike traditional MCMC methods such as Metropolis–Hastings, which rely on inefficient random-walk proposals, HMC leverages concepts from Hamiltonian dynamics in physics to explore the parameter space more efficiently. The following HMC algorithm accepts or rejects the candidate state at the end of each trajectory.

---

#### Algorithm 1 Hamiltonian Monte Carlo (HMC)

---

**Target:** Generate a Markov chain  $(\boldsymbol{\theta}^{(i)}, \mathbf{r}^{(i)})$  for  $i = 1$  to  $M$  with posterior density  $\pi(\boldsymbol{\theta}) \propto \exp\{\ell(\boldsymbol{\theta})\}$ .

1. Set the current position  $\boldsymbol{\theta}_0 = \boldsymbol{\theta}^{(i)}$  and draw  $\mathbf{r}^0 \sim \mathcal{N}_p(0, \mathbf{I}_p)$ .
2. Simulate a trajectory via the leapfrog steps starting from  $(\boldsymbol{\theta}_0, \mathbf{r}_0)$  by applying  $L$  leapfrog updates of step size  $\epsilon$ .

$$\tilde{\mathbf{r}} \leftarrow \mathbf{r} + (\epsilon/2)\nabla_{\boldsymbol{\theta}}\ell(\boldsymbol{\theta}),$$

$$\tilde{\boldsymbol{\theta}} \leftarrow \boldsymbol{\theta} + \epsilon\tilde{\mathbf{r}},$$

$$\tilde{\mathbf{r}} \leftarrow \tilde{\mathbf{r}} + (\epsilon/2)\nabla_{\boldsymbol{\theta}}\ell(\tilde{\boldsymbol{\theta}}),$$

3. Accept with probability

$$\alpha = \min\left(1, \frac{\exp(\ell(\tilde{\boldsymbol{\theta}}) - \frac{1}{2}\tilde{\mathbf{r}} \cdot \tilde{\mathbf{r}})}{\exp(\ell(\boldsymbol{\theta}^{(i-1)}) - \frac{1}{2}\mathbf{r}_0 \cdot \mathbf{r}_0)}\right)$$

If accepted, set  $(\boldsymbol{\theta}^{(i+1)}, \mathbf{r}^{(i+1)}) = (\tilde{\boldsymbol{\theta}}, \tilde{\mathbf{r}})$ ; otherwise set  $(\boldsymbol{\theta}^{(i+1)}, \mathbf{r}^{(i+1)}) = (\boldsymbol{\theta}^{(i)}, \mathbf{r}^{(i)})$ .

---

The three models (SLn, SLt, SLcn) differ in their error distributions, which yield different forms of the log-likelihood. This log-likelihood, combined with the prior distributions, defines the joint log-posterior  $\ell(\boldsymbol{\theta})$ . We note that  $\boldsymbol{\theta}$  comprises all model parameters (e.g.,  $\boldsymbol{\theta} = (\beta, \gamma, \sigma^2, \rho)$  in the SLn model),  $\epsilon$  denotes the leapfrog step size,  $L$  the number of leapfrog steps,  $M$  the total number of iterations, and  $\mathbf{r}$  the auxiliary momentum variable introduced in HMC. The HMC algorithm only requires the log-target  $\ell(\boldsymbol{\theta})$  and its gradient  $\nabla_{\boldsymbol{\theta}}\ell(\boldsymbol{\theta})$ ; a momentum variable is introduced, leapfrog integration with step size  $\epsilon$  is performed for  $L$  steps, and a Metropolis–Hastings correction determines the acceptance probability  $\alpha$ .

Although  $\epsilon$ ,  $L$ , and  $M$  are theoretically key tuning parameters in HMC, Stan’s NUTS implementation automatically adapts  $\epsilon$  and the effective trajectory length (replacing a fixed  $L$ ), while the user only specifies the total number of iterations  $M$ . Thus, the only model-specific component to implement is the log-posterior, whereas HMC itself operates uniformly to draw posterior samples.

## Pseudo-code for SLn Model

---

**Algorithm 2** Posterior Sampling for SLn Model via HMC

---

**Require:** Data  $(Y, X, W)$ , prior hyperparameters

- 1: Define parameter vector  $\boldsymbol{\theta} = (\beta, \gamma, \sigma^2, \rho)$
  - 2: Specify priors:
    - $\beta \sim \mathcal{N}(0, 10^2 I)$ ,  $\gamma \sim \mathcal{N}(0, 10^2 I)$
    - $\sigma^2 \sim \text{Cauchy}(0, 5)$ ,  $\rho \sim \text{Uniform}(-1, 1)$
  - 3: Compute the posterior distribution  $\pi_{\text{SLn}}(\boldsymbol{\theta} \mid \mathbf{y})$  based on the priors and likelihood in (16).
  - 4: Run HMC in Algorithm1 using  $\pi(\boldsymbol{\theta})$  to draw posterior samples
- 

## Pseudo-code for SLt Model

---

**Algorithm 3** Posterior Sampling for SLt Model via HMC

---

**Require:** Data  $(Y, X, W)$ , prior hyperparameters

- 1: Define parameter vector  $\boldsymbol{\theta} = (\beta, \gamma, \sigma^2, \rho, \nu)$
  - 2: Specify priors:
    - $\beta \sim \mathcal{N}(0, 10^2 I)$ ,  $\gamma \sim \mathcal{N}(0, 10^2 I)$
    - $\sigma^2 \sim \text{Cauchy}(0, 5)$ ,  $\rho \sim \text{Uniform}(-1, 1)$
    - $\nu \sim \text{Gamma}(2, 0.1)$
  - 3: Compute the posterior distribution  $\pi_{\text{SLt}}(\boldsymbol{\theta} \mid \mathbf{y})$  based on the priors and likelihood in (17).
  - 4: Run HMC in Algorithm1 using  $\pi(\boldsymbol{\theta})$  to draw posterior samples
- 

## Pseudo-code for SLcn Model

---

**Algorithm 4** Posterior Sampling for SLcn Model via HMC

---

**Require:** Data  $(Y, X, W)$ , prior hyperparameters

- 1: Define parameter vector  $\boldsymbol{\theta} = (\beta, \gamma, \sigma^2, \rho, \nu_1, \nu_2)$
  - 2: Specify priors:
    - $\beta \sim \mathcal{N}(0, 10^2 I)$ ,  $\gamma \sim \mathcal{N}(0, 10^2 I)$
    - $\sigma^2 \sim \text{Cauchy}(0, 5)$ ,  $\rho \sim \text{Uniform}(-1, 1)$
    - $\nu_1 \sim \text{Beta}(1, 1)$ ,  $\nu_2 \sim \text{Beta}(1, 1)$
  - 3: Compute the posterior distribution  $\pi_{\text{SLcn}}(\boldsymbol{\theta} \mid \mathbf{y})$  based on the priors and likelihood in (18).
  - 4: Run HMC in Algorithm1 using  $\pi(\boldsymbol{\theta})$  to draw posterior samples
- 

**Implementation:** Full Stan implementations for the three models are available at:

- SLn : <https://github.com/heeju-lim/HeckmanStan/blob/master/inst/stan/HeckmanNormal.stan>
- SLt : <https://github.com/heeju-lim/HeckmanStan/blob/master/inst/stan/HeckmanT.stan>
- SLCn : <https://github.com/heeju-lim/HeckmanStan/blob/master/inst/stan/HeckmanCNormal.stan>

### S.3 Posterior Diagnostics

To evaluate the quality and convergence of the posterior samples generated via Hamiltonian Monte Carlo (HMC), we examine three standard diagnostic criteria across all three models (SLn, SLt, SLCn): (1) the potential scale reduction factor (R-hat), (2) the effective sample size (ESS), and (3) the acceptance rate.

All R-hat values are close to 1.00, indicating that the Markov chains have converged well. The effective sample sizes (ESS) are sufficiently large for all parameters, ensuring that the Monte Carlo error is negligible. Additionally, the acceptance rate across simulations remains within the ideal range (typically 0.88–0.92), reflecting stable HMC performance.

We summarize these diagnostics in Table S.3.1, presenting the mean R-hat, mean ESS across 100 replicates, and acceptance rate for each model when the sample size is 400 and the data are generated from the Student’s-t distribution.

Table S.3.1: Posterior diagnostics across 100 replicates. Reported are the mean R-hat, mean effective sample size (ESS), and Acceptance Rate.

| Distribution    | Parameter  | SLn   |      | SLt   |      | SLCn  |      |
|-----------------|------------|-------|------|-------|------|-------|------|
|                 |            | R-hat | ESS  | R-hat | ESS  | R-hat | ESS  |
| Student’s-t     | $\beta_1$  | 1.00  | 3563 | 1.00  | 3659 | 1.00  | 3647 |
|                 | $\beta_2$  | 1.00  | 3714 | 1.00  | 3705 | 1.00  | 3724 |
|                 | $\gamma_1$ | 1.00  | 3727 | 1.00  | 3636 | 1.00  | 3508 |
|                 | $\gamma_2$ | 1.00  | 3731 | 1.00  | 3666 | 1.00  | 3638 |
|                 | $\gamma_3$ | 1.00  | 3710 | 1.00  | 3680 | 1.00  | 3638 |
|                 | $\sigma^2$ | 1.00  | 3655 | 1.00  | 3635 | 1.00  | 3540 |
|                 | $\rho$     | 1.00  | 3541 | 1.00  | 3675 | 1.00  | 3656 |
|                 | $\nu$      |       |      | 1.00  | 3613 |       |      |
|                 | $\nu_1$    |       |      |       |      | 1.00  | 3518 |
|                 | $\nu_2$    |       |      |       |      | 1.00  | 3627 |
| Acceptance Rate |            | 0.90  |      | 0.88  |      | 0.91  |      |

### S.4 Correlation Matrix of Posterior Distributions

In this section, we present several figures illustrating the properties of the SLCn model, including the correlation structure of posterior distributions in the outcome equation.

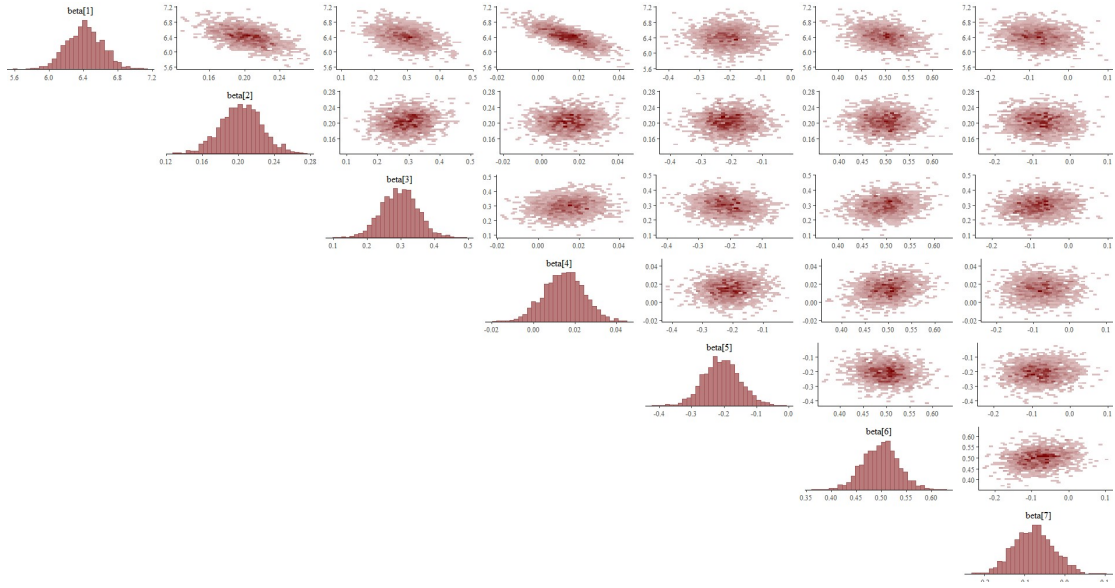

Figure S.4.3: Ambulatory expenditure data. Correlation of posterior distributions for beta parameters of SLcn model in outcome equation.

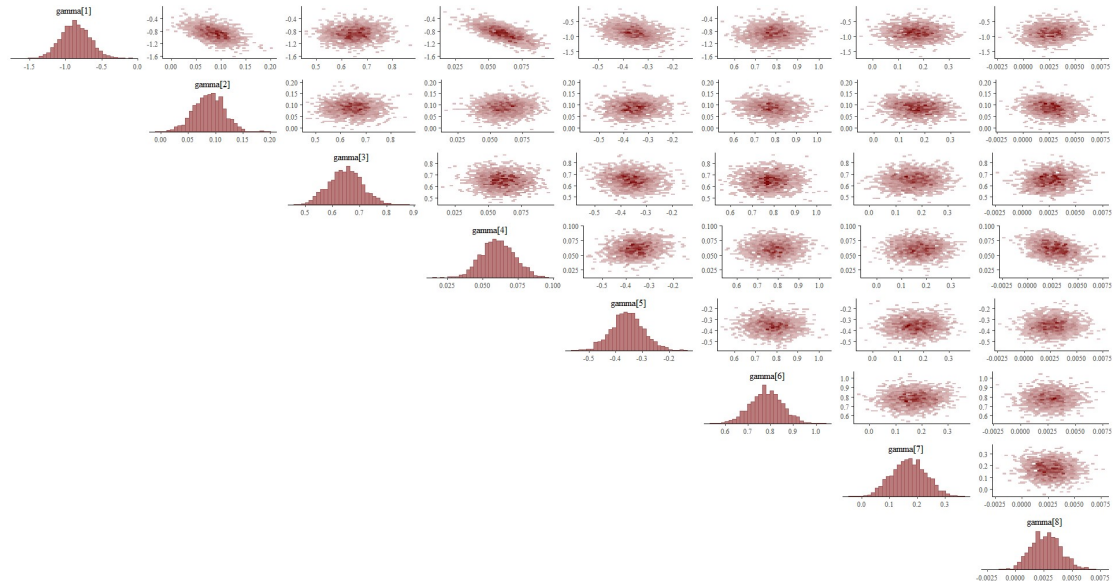

Figure S.4.4: Ambulatory expenditure data. Correlation of posterior distributions for gamma parameters of SLcn model in selection equation

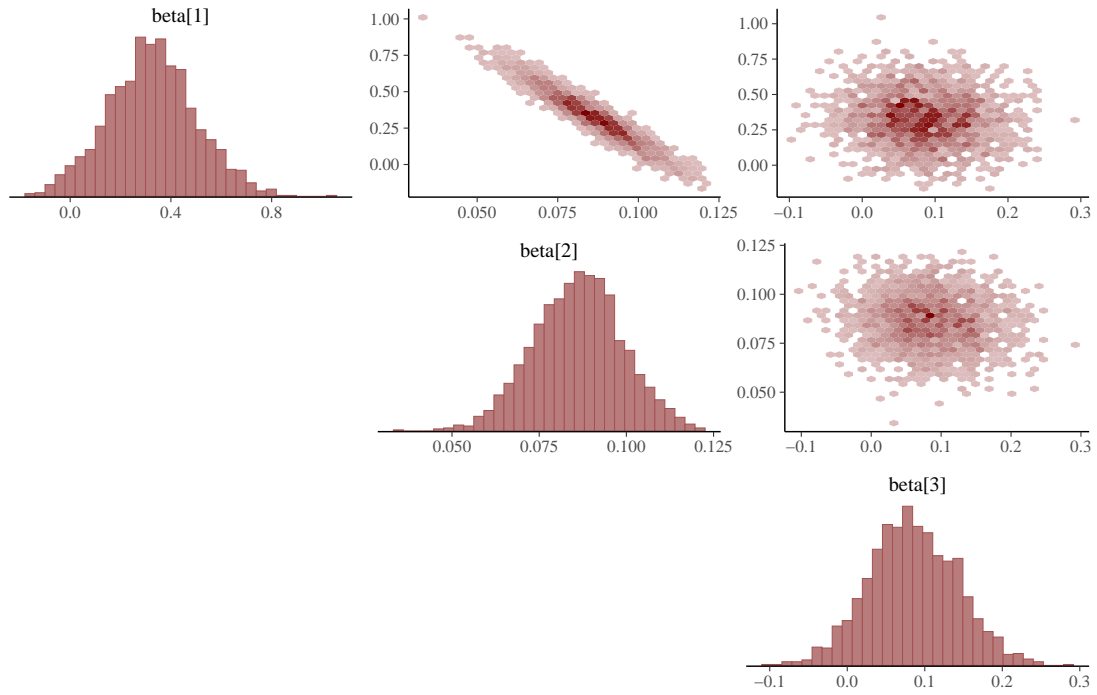

Figure S.4.5: Mroz: Labor Supply Data. Correlation of posterior distributions for beta parameters of SLcn model in outcome equation

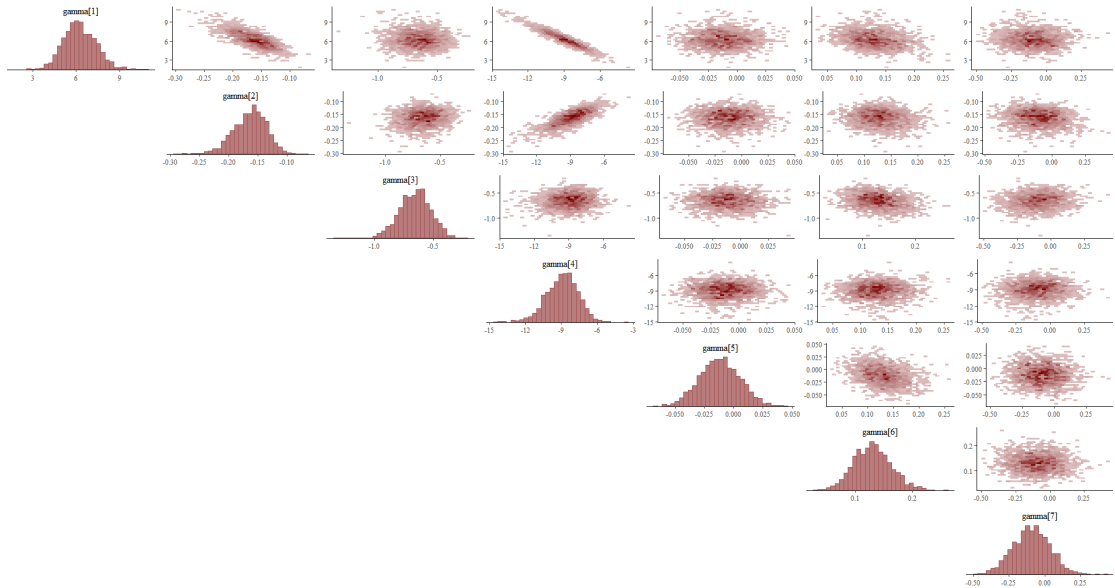

Figure S.4.6: Mroz: Labor Supply Data. Correlation of posterior distributions for gamma parameters of SLcn model in selection equation
